# Supplementary material for: Tackling Data Corruption in Offline Reinforcement Learning via Sequence Modeling
Source: arXiv:2407.04285 source file (2025-03-02)
Supplement: Supplementary file 1 [file theory.tex]

Before we provide our theoretical analysis, we first introduce some necessary notions. 
In our analysis, we consider an episodic setting with the episode length of $H$.
We denote the visited state-action history as $\tau_h = (s_0,a_0,s_1,a_1,\cdots,s_h,a_h)$. The reward at $h$-th step is $r_h(s_h,a_h)$, where $s_h\in\mathcal S$ and $a_h\in\mathcal A$.
Reward-to-go serves as a condition variable for the policy, denoted as $R_h$, that is the reward-to-go at the $h$-th step. For abbreviation, we let $R_{1:h}$ denote a sequence of reward-to-go from step $1$ to step $h$, which is $(R_1,\ldots,R_h)$. 
We consider a history-dependent policy conditioned on the reward-to-go, denoted as $\pi(a_h| \tau_h;R_{1:h})$, which is the probability of generating the action $a_h$.

We assume that $\mathcal{D}$ is a dataset which is generated by a behavior policy $\pi_h^b(\cdot| \tau_h;R_{1:h}^b)$ under a certain reward-to-go sequence $R_{1:h}^b$. We let $\mathbf{P}^b(\cdot;R^b_{1:H})$ be the joint distribution for $\tau_H = (s_1, a_1,\cdots, s_H, a_H)$ induced by a corrupted-equivalent transition model $\mathbb{P}_h(s'|s,a)$ and the behavior policy $\pi_h^b(\cdot| \tau_h;R_{1:h}^b)$ for all $h\in[H]$.

We further assume that $\tilde{\mathcal{D}}$ is generated by a corrupted-equivalent behavior policy $\tilde{\pi}_h^b(\cdot| \tau_h;\tilde R_{1:h}^b)$ under some certain $\tilde{R}_{1:h}^b$. And $\tilde{\mathbf{P}}^b(\cdot;\tilde R^b_{1:H})$ is the joint distribution for $\tilde\tau_H = (\tilde s_1,\tilde a_1,\cdots,\tilde s_H,\tilde a_H)$ induced by the transition model $\tilde{\mathbb{P}}_h(s'|s,a)$ and the behavior policy $\tilde\pi_h^b(\cdot| \tilde\tau_h;\tilde R_{1:h}^b)$ for all $h\in[H]$.

Denoting the value function as $V^\pi = \mathbb{E}_{\pi,\mathbb{P}} [ \sum_{h=1}^H r_h(s_h,a_h) ]$ defined on the true reward funtion $r_h$. We assume that there exists an optimal policy 
\begin{align*}
\pi^* = \argmax_\pi V^\pi,
\end{align*}
where $\pi^*$ is in the form of
\begin{align*}
    \pi_h^*(a_h|\tau_h;R_{1:h}^*)
\end{align*}
where $R_{1:h}^*$ is a reward-to-go sequence  from step $1$ to step $h$, leading to an optimal policy.

%
%
%
%We assume that $\theta^*$ is the optimal solution to the following optimization problem under the uncorrupted data,
%\begin{align}
%    \hat{\theta} := \argmax_{\theta\in\Theta} \mathbb{E}_\mathcal{D} \sum_{h=1}^H \log \pi_\theta(a_h|\tau_h;R_{1:h}),\label{eq:uncorrupt-mle}
%\end{align}
We assume that $\hat{\theta}$ is the learned solution to the following optimization problem based the corrupted data $\tilde{\mathcal{D}}$: 
\begin{align}
    \hat{\theta} := \argmax_{\theta\in\Theta} \mathbb{E}_{\tilde{\mathcal{D}}} \sum_{h=1}^H \log\pi_\theta(a_h|\tau_h;\hat{R}_{1:h}), \label{eq:corrupt-mle}
\end{align}

\begin{align}
    \tilde\theta := \argmax_{\theta\in\Theta} \mathbb{E}_{\tilde{\mathcal{D}}} \sum_{h=1}^H \log\pi_\theta(a_h|\tau_h;\tilde R_{1:h}^b), \label{eq:corrupt-mle-2}
\end{align}

%For \eqref{eq:uncorrupt-mle}, we have
%\begin{align*}
% \frac{1}{2}\left\|\mathbf{P}_{\hat{\theta}}(\cdot;R_{1:H}) - \mathbf{P}^b(\cdot; R^b_{1:H})\right\|_{\mathrm{TV}}^2 \leq \left\|\sqrt{\mathbf{P}_{\hat{\theta}}(\cdot;R_{1:H})} - \sqrt{\mathbf{P}^b(\cdot; R^b_{1:H})}\right\|_2^2 \leq     \frac{\log(|\Theta|/\delta)}{N} 
%\end{align*}

For Eq.~\ref{eq:corrupt-mle} and Eq.~\ref{eq:corrupt-mle-2}, we have
\begin{align*}
 \frac{1}{2}\left\|\tilde{\mathbf{P}}_{\tilde{\theta}}(\cdot;\tilde R_{1:H}) - \tilde{\mathbf{P}}^b(\cdot;\tilde R^b_{1:H})\right\|_{\mathrm{TV}}^2 \leq \left\|\sqrt{\mathbf{P}_{\tilde{\theta}}(\cdot;\tilde R_{1:H})} - \sqrt{\tilde{\mathbf{P}}^b(\cdot; \tilde R^b_{1:H})}\right\|_2^2 \leq     \frac{\log(|\Theta|/\delta)}{N} 
\end{align*}

We consider the following decomposition
\begin{align*}
    V^{\pi^*} - V^{\pi_{\tilde{\theta}}} &=V^{\pi^*} - V^{\pi^b} + V^{\pi^b} - V^{\tilde{\pi}^b} + V^{\tilde{\pi}^b}- V^{\pi_{\tilde{\theta}}}
\end{align*}

We consider the following difference
\begin{align*}
    &V^{\pi^*} -  V^{\pi^b} \\
    &\leq \sum_{\tau_H\in \mathcal{S}^H\times\mathcal{A}^H}\left(\sum_{h=1}^H r_h(s_h,a_h)\right)\left(\mathbf{P}^*(\tau_H;R_{1:H}^*) - \mathbf{P}^b(\tau_H; R_{1:H}^b)\right)\\
    &\leq 2H\left\|\mathbf{P}^*(\cdot;R_{1:H}^*) - \mathbf{P}^b(\cdot; R_{1:H}^b)\right\|_{\mathrm{TV}} 
\end{align*}
where we assume that $|r_h(s,a)|\leq 1$.

We consider the following difference
\begin{align*}
    &V^{\pi^b} -  V^{\tilde\pi^b} \\
    &\leq \sum_{\tau_H\in \mathcal{S}^H\times\mathcal{A}^H}\left(\sum_{h=1}^H r_h(s_h,a_h)\right)\left(\mathbf{P}^b(\tau_H;R_{1:H}^b) - \tilde{\mathbf{P}}^b(\tau_H; \tilde R_{1:H}^b)\right)\\
    &\leq 2H\left\|\mathbf{P}^b(\tau_H;R_{1:H}^b) - \tilde{\mathbf{P}}^b(\tau_H; \tilde R_{1:H}^b)\right\|_{\mathrm{TV}} 
\end{align*}
where we assume that $|r_h(s,a)|\leq 1$.

We consider the following difference
\begin{align*}
    &V^{\tilde\pi^b} -  V^{\pi_{\tilde{\theta}}} \\
    &\leq \sum_{\tau_H\in \mathcal{S}^H\times\mathcal{A}^H}\left(\sum_{h=1}^H r_h(s_h,a_h)\right)\left(\tilde{\mathbf{P}}^b(\tau_H;\tilde{R}_{1:H}^b) - \mathbf{P}_{\tilde{\theta}}(\tau_H;\tilde R_{1:H})\right)\\
    &\leq 2H\left\|\tilde{\mathbf{P}}^b(\tau_H;\tilde{R}_{1:H}^b) - \mathbf{P}_{\tilde{\theta}}(\tau_H;\tilde R_{1:H})\right\|_{\mathrm{TV}}\\
    &\leq 2H\sqrt{\frac{2\log(|\Theta|/\delta)}{N}}  
\end{align*}
where we assume that $|r_h(s,a)|\leq 1$.

% We consider the following difference
% \begin{align*}
%     &V^{\pi_{\hat{\theta}}} -  V^{\pi_{\tilde{\theta}}} \\
%     &\leq \sum_{\tau_H\in \mathcal{S}^H\times\mathcal{A}^H}\left(\sum_{h=1}^H r_h(s_h,a_h)\right)\left(\mathbf{P}_{\hat{\theta}}(\tau_H;R_{1:H}) - \mathbf{P}_{\tilde{\theta}}(\tau_H;\tilde R_{1:H})\right)\\
%     &\leq 2H\left\|\mathbf{P}_{\hat{\theta}}(\cdot;R_{1:H}) - \mathbf{P}_{\tilde{\theta}}(\cdot;\tilde R_{1:H})\right\|_{\mathrm{TV}}\\
%     &\leq 2H\left\|\mathbf{P}_{\hat{\theta}}(\cdot;R_{1:H}) - \mathbf{P}^b(\cdot; R^b_{1:H})\right\|_{\mathrm{TV}} + 2H\left\|\mathbf{P}^b(\cdot; R^b_{1:H}) - \tilde{\mathbf{P}}^b(\cdot; \tilde R^b_{1:H})\right\|_{\mathrm{TV}} + 2H\left\|\tilde{\mathbf{P}}^b(\cdot; \tilde R^b_{1:H}) - \mathbf{P}_{\tilde{\theta}}(\cdot;\tilde R_{1:H})\right\|_{\mathrm{TV}}\\
%     &\leq 4H\sqrt{\frac{2\log(|\Theta|/\delta)}{N}}  + 2H\left\|\mathbf{P}^b(\cdot; R^b_{1:H}) - \tilde{\mathbf{P}}^b(\cdot; \tilde R^b_{1:H})\right\|_{\mathrm{TV}} 
% \end{align*}

Furthermore, we have
\begin{align*}
    &\left\|\mathbf{P}^b(\cdot; R^b_{1:H}) - \tilde{\mathbf{P}}^b(\cdot; \tilde R^b_{1:H})\right\|_{\mathrm{TV}} \\
    & \leq \sqrt{ \mathbb{E}_{\tau_H \sim \mathbf{P}^b(\cdot; R^b_{1:H})}\log\frac{\mathbf{P}^b(\tau_H; R^b_{1:H})}{\tilde{\mathbf{P}}^b(\tau_H; \tilde R^b_{1:H})}}\\
    & \leq \sqrt{ C \mathbb{E}_{\tau_H \sim \mathbf{P}^\mathcal{D}(\cdot)}\log\frac{\mathbf{P}^b(\tau_H; R^b_{1:H})}{\tilde{\mathbf{P}}^b(\tau_H; \tilde R^b_{1:H})}}\\
    &= \sqrt{ C \frac{1}{N}\sum_{i=1}^N\log\frac{\mathbf{P}^b(\tau_H^{(i)}; R^b_{1:H})}{\tilde{\mathbf{P}}^b(\tau_H^{(i)}; \tilde R^b_{1:H})}}\\
    &= \sqrt{ C \frac{1}{N}\sum_{i=1}^N\sum_{h=1}^H\log\frac{\pi_h^b(\tau_h^{(i)}; R^b_{1:h})}{\tilde{\pi}^b(\tau_h^{(i)}; \tilde R^b_{1:h})}}\\
    &\leq \sqrt{ C \frac{\zeta}{N}}
\end{align*}
where the coverage assumption $\sup_{\tau_H}\mathbf{P}^b(\tau_H; R^b_{1:H})/\mathbf{P}^{\tilde{\mathcal{D}}}(\tau_H)\leq C$ and the corruption $\sum_{i=1}^N\sum_{h=1}^H\log\frac{\pi_h^b(\tau_h^{(i)}; R^b_{1:h})}{\tilde{\pi}^b(\tau_h^{(i)}; \tilde R^b_{1:h})} \leq \zeta$

% We have the following decomposition for the value function
% \begin{align*}
% V^{\pi^*} - V^{\pi_{\hat{\theta}}} \leq \underbrace{V^{\pi^*} - V^{\pi_{\theta^*}}}_{\text{intrinsic error}} + \underbrace{V^{\pi_{\theta^*}} - V^{\pi_{\hat{\theta}}}}_{\text{corruption error}}
% \end{align*}

% The intrinsic error is the error induced by applying the decision transformer model to solve POMDP, which can be directly bounded by a constant error $\mathcal{E}_{\mathrm{DT}}$. If the decision transformer model is sufficiently good, then probably $\mathcal{E}_{\mathrm{DT}} = 0$ can be satisfied:
% \begin{align*}
% V^{\pi^*} - V^{\pi_{\theta^*}} \leq \mathcal{E}_{\mathrm{DT}}
% \end{align*}

% We focus on bounding the error induced by corruption:
% \begin{align*}
% V^{\pi_{\theta^*}} - V^{\pi_{\hat{\theta}}} \leq 
% \end{align*}
